# Supplementary material for: Kepler: Robust Learning for Faster Parametric Query Optimization
Source: arXiv:2306.06798 source file (2023-10-18)
Supplement: Supplementary file 1 [file Appendix.tex]

\appendix

\section{Experiment Configuration}

\paragraph{Row Count Evolution}

Furthermore, our implementation of RCE only perturbs join cardinality estimates, and ignores base table estimates, due to lack of functionality in pg\_hint\_plan. As a result, we rely on parameter binding values to provide diversity over base table scan methods in the candidate plan set. 

\section{Sub-plan cardinality computation with timeouts}

\section{Additional figures}

\begin{figure*}[!t]
    \centering
    \includegraphics[scale=0.43]{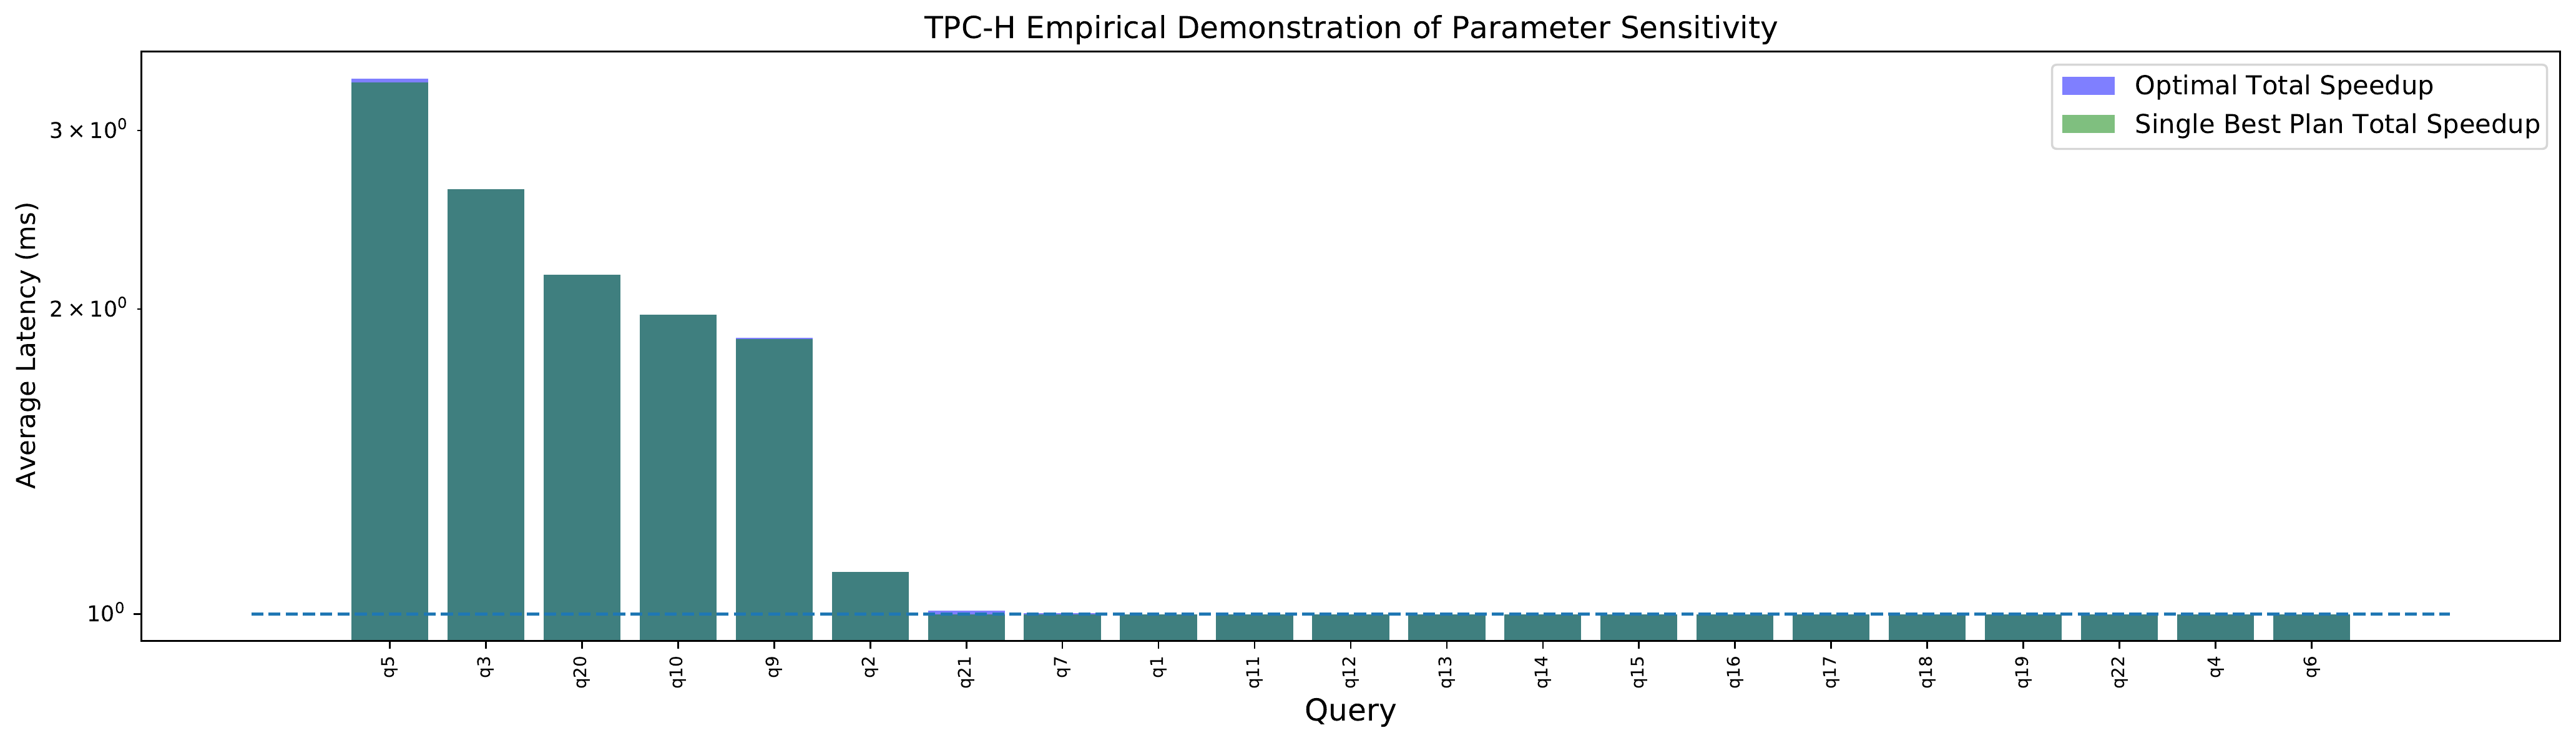}
    \caption{TPC-H queries are not parameter sensitive as an optimal strategy that considers multiple plans provides the same latency gains as using a single-best-plan strategy. Dashed line corresponds to speedup ratio 1, i.e. no improvement over the existing query optimizer.}
    \label{fig:tpch_single_best_plan}
\end{figure*}

\begin{figure*}[!t]
    \centering
    \includegraphics[scale=0.43]{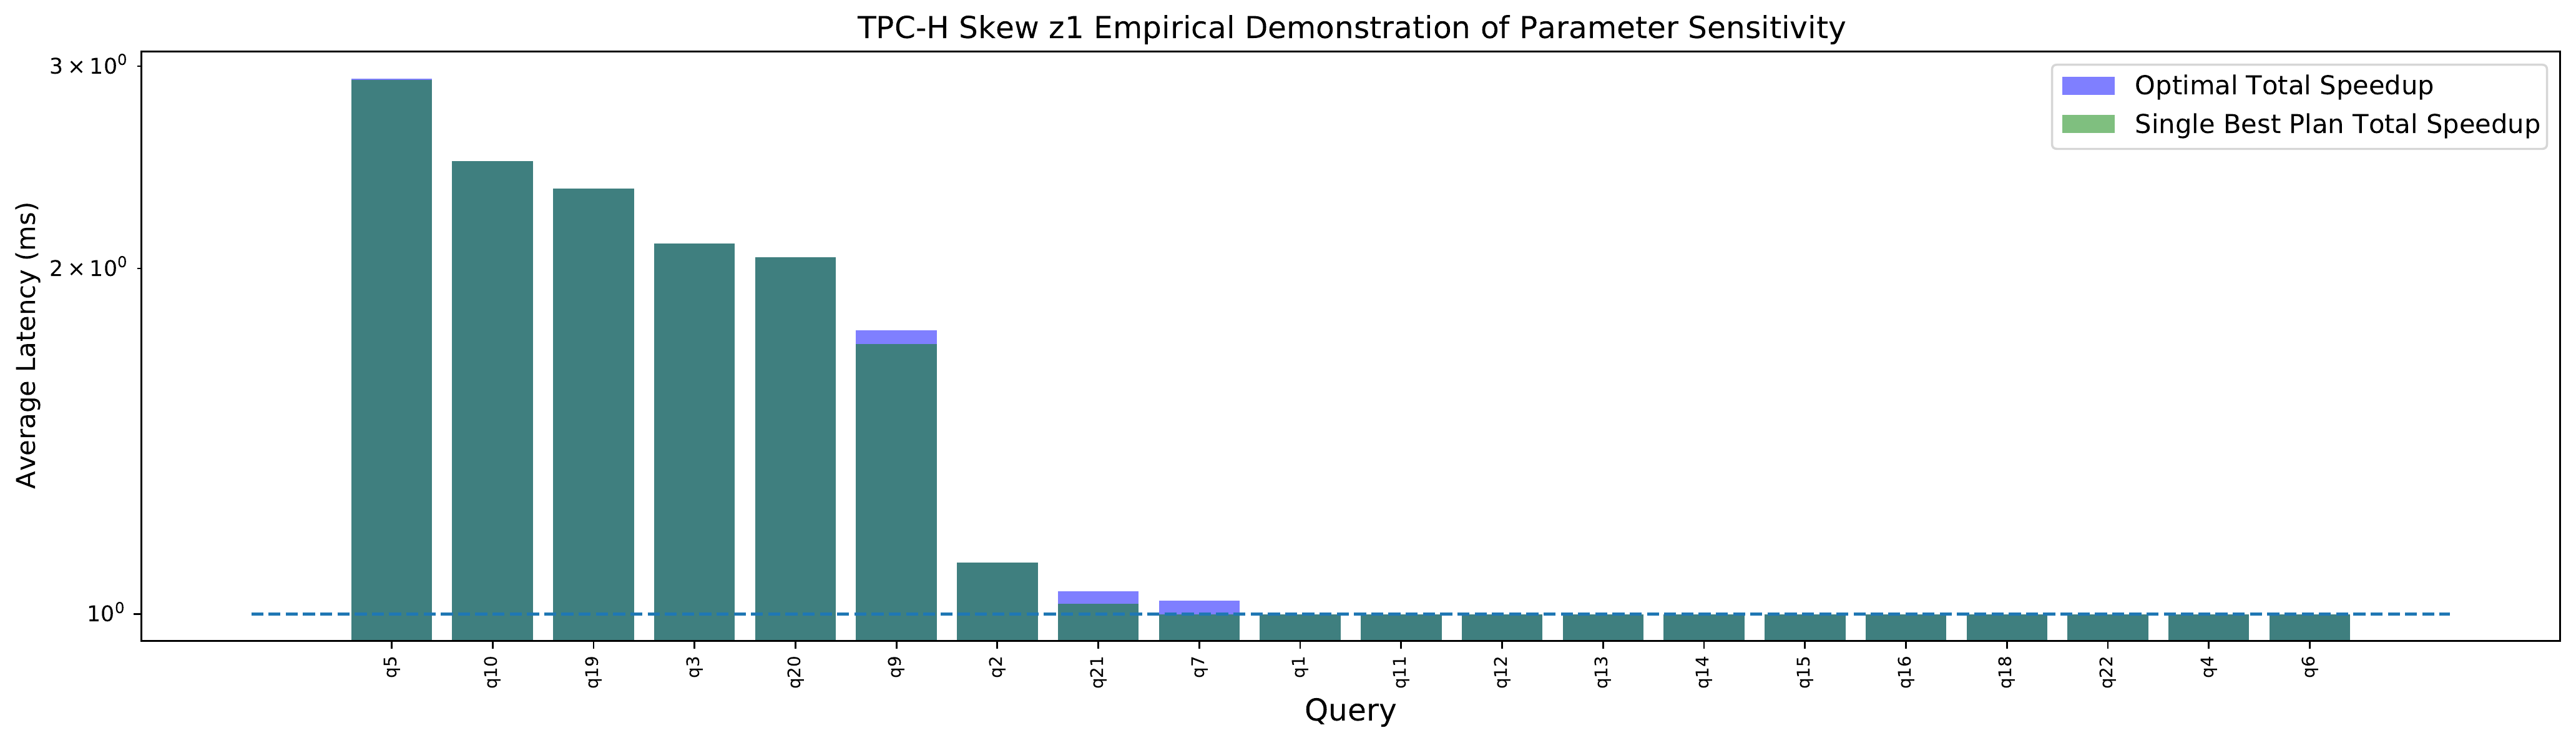}
    \caption{TPC-H Skew z1 queries are not meaningfully parameter sensitive as an optimal strategy that considers multiple plans provides the same latency gains as using a single-best-plan strategy. Dashed line corresponds to speedup ratio 1, i.e. no improvement over the existing query optimizer.}
    \label{fig:tpch_skew1_single_best_plan}
\end{figure*}
